# Supplementary material for: Pose Guided Person Image Generation
Source: arXiv:1705.09368 source file (2018-01-28)
Supplement: Supplementary file 1 [file 1-supp-arch.tex]

\section{Network architecture}
In this section, we give the details of our network architecture. Since images in the two datasets have different resolutions, we use slightly different network architecture for them. On the Market-1501 dataset, for generator at stage-I G1, the encoder consists of five residual blocks and one fully-connected layer. The decoder is symmetric to the decoder except for the last layer that generates an image of 3 channels. The network is shown in Figure~\ref{fig:G1_net}. 
Each residual block in the network consists of two convolution layers with stride=1 followed by one convolution layer with stride=2 for downsampling except the last block, which is shown in Figure~\ref{fig:res_block}. 

For generator at stage-II G2, it has similar network architecture to G1 but only three residual blocks in the encoder and decoder, as shown in Figure~\ref{fig:G2_net}

On the DeepFashion dataset, since the input image has a size of 256$\times$256, we use one more residual block than the one used on Market-1501 dataset. That is, we have six residual blocks for encoder and decoder in G1 and four residual blocks for encoder and decoder in G2.

\begin{figure}[hbtp]
\centering
	\includegraphics[width=1\linewidth]{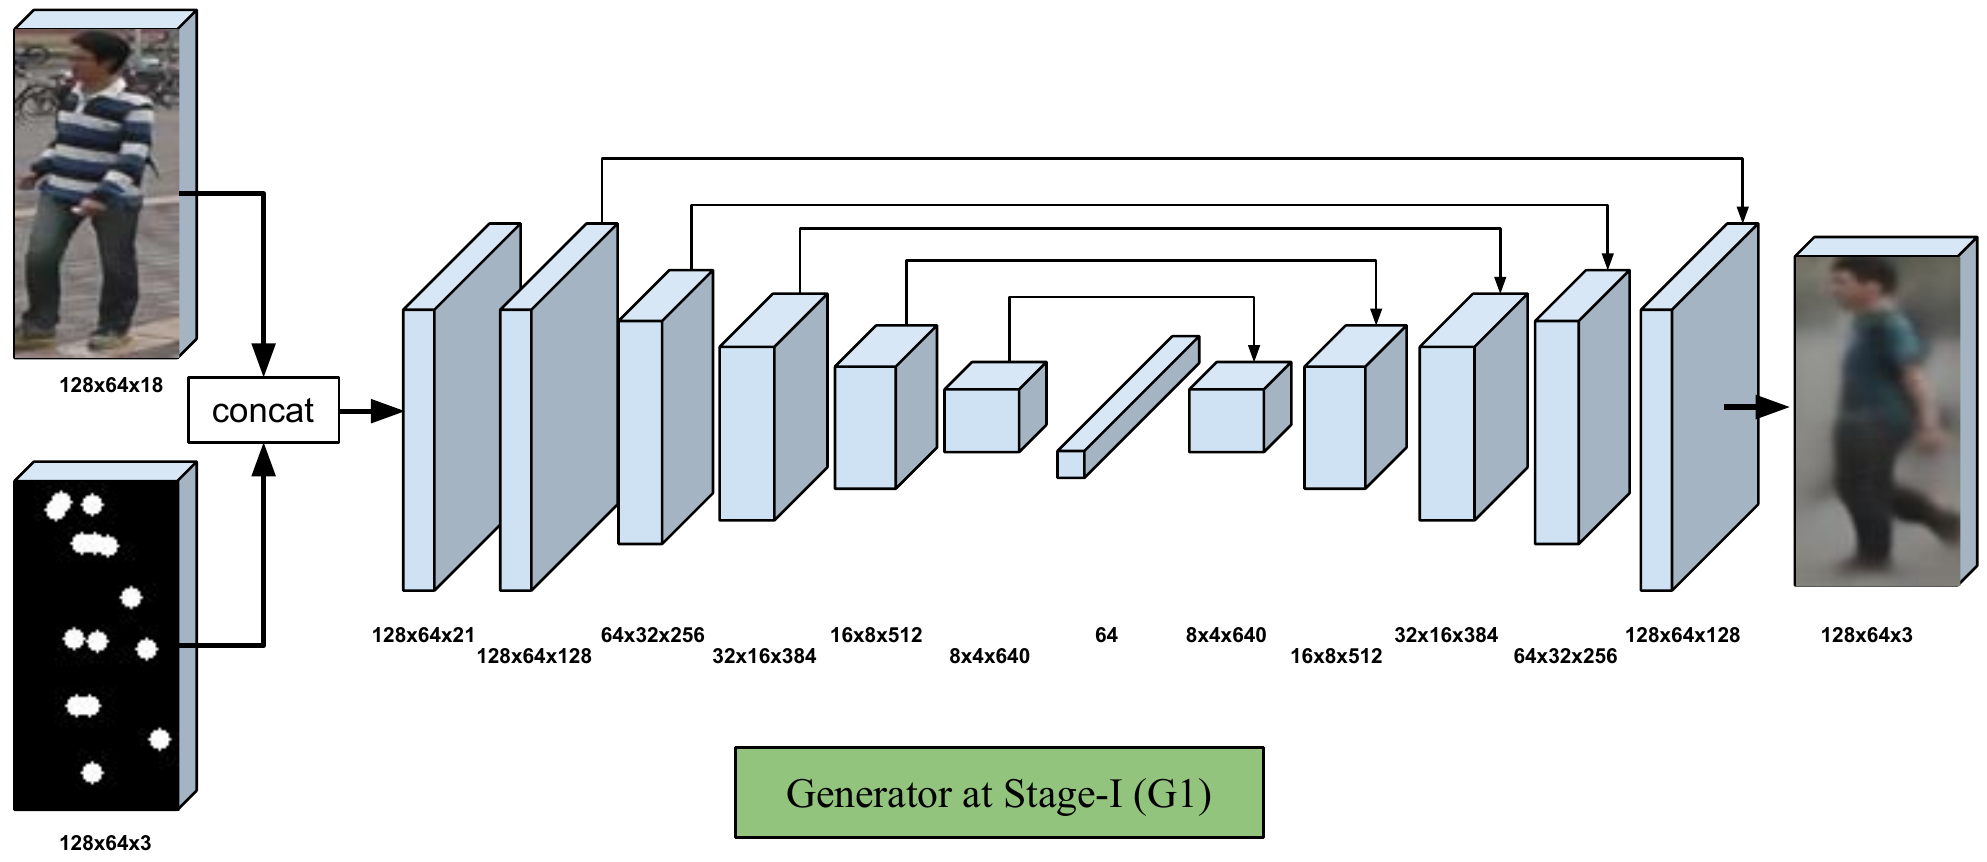}
    \caption{Network architecture of generator at stage-I.}
    \label{fig:G1_net}
    \vspace{-2mm}
\end{figure}

\begin{figure}[hbtp]
\centering
	\includegraphics[width=0.9\linewidth]{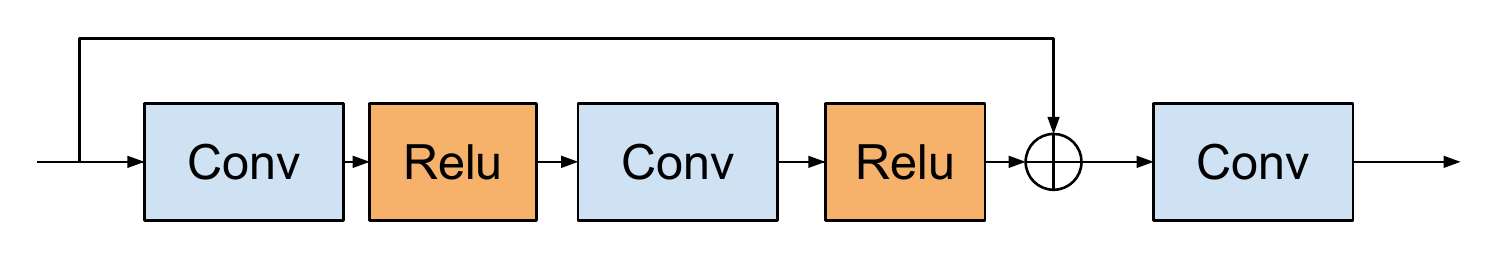}
    \caption{Residual block.}
    \label{fig:res_block}
\end{figure}
 
\begin{figure}[htbp]
\centering
	\includegraphics[width=0.8\linewidth]{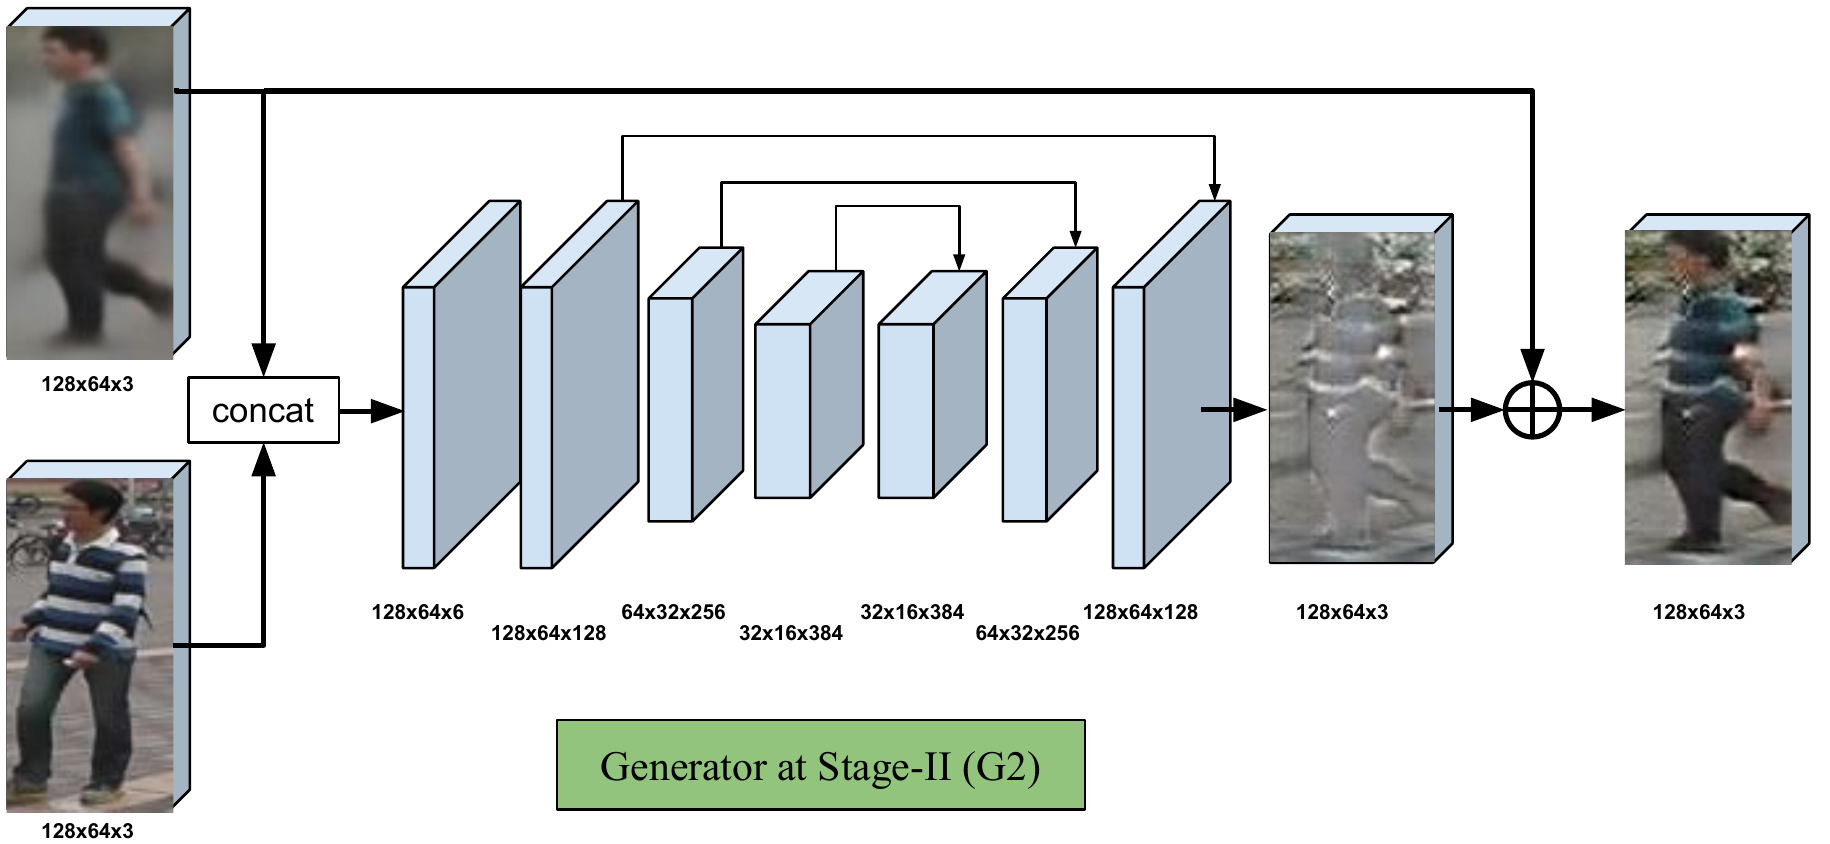}
    \caption{Network architecture of generator at stage-II.}
    \label{fig:G2_net}
\end{figure}
