# Supplementary material for: Pose Guided Person Image Generation
Source: arXiv:1705.09368 source file (2018-01-28)
Supplement: Supplementary file 3 [file 3-supp-seq.tex]

\section{Person image generation of arbitrary poses}
\label{supp-seq}

\begin{figure}
\centering
  \includegraphics[width=\linewidth]{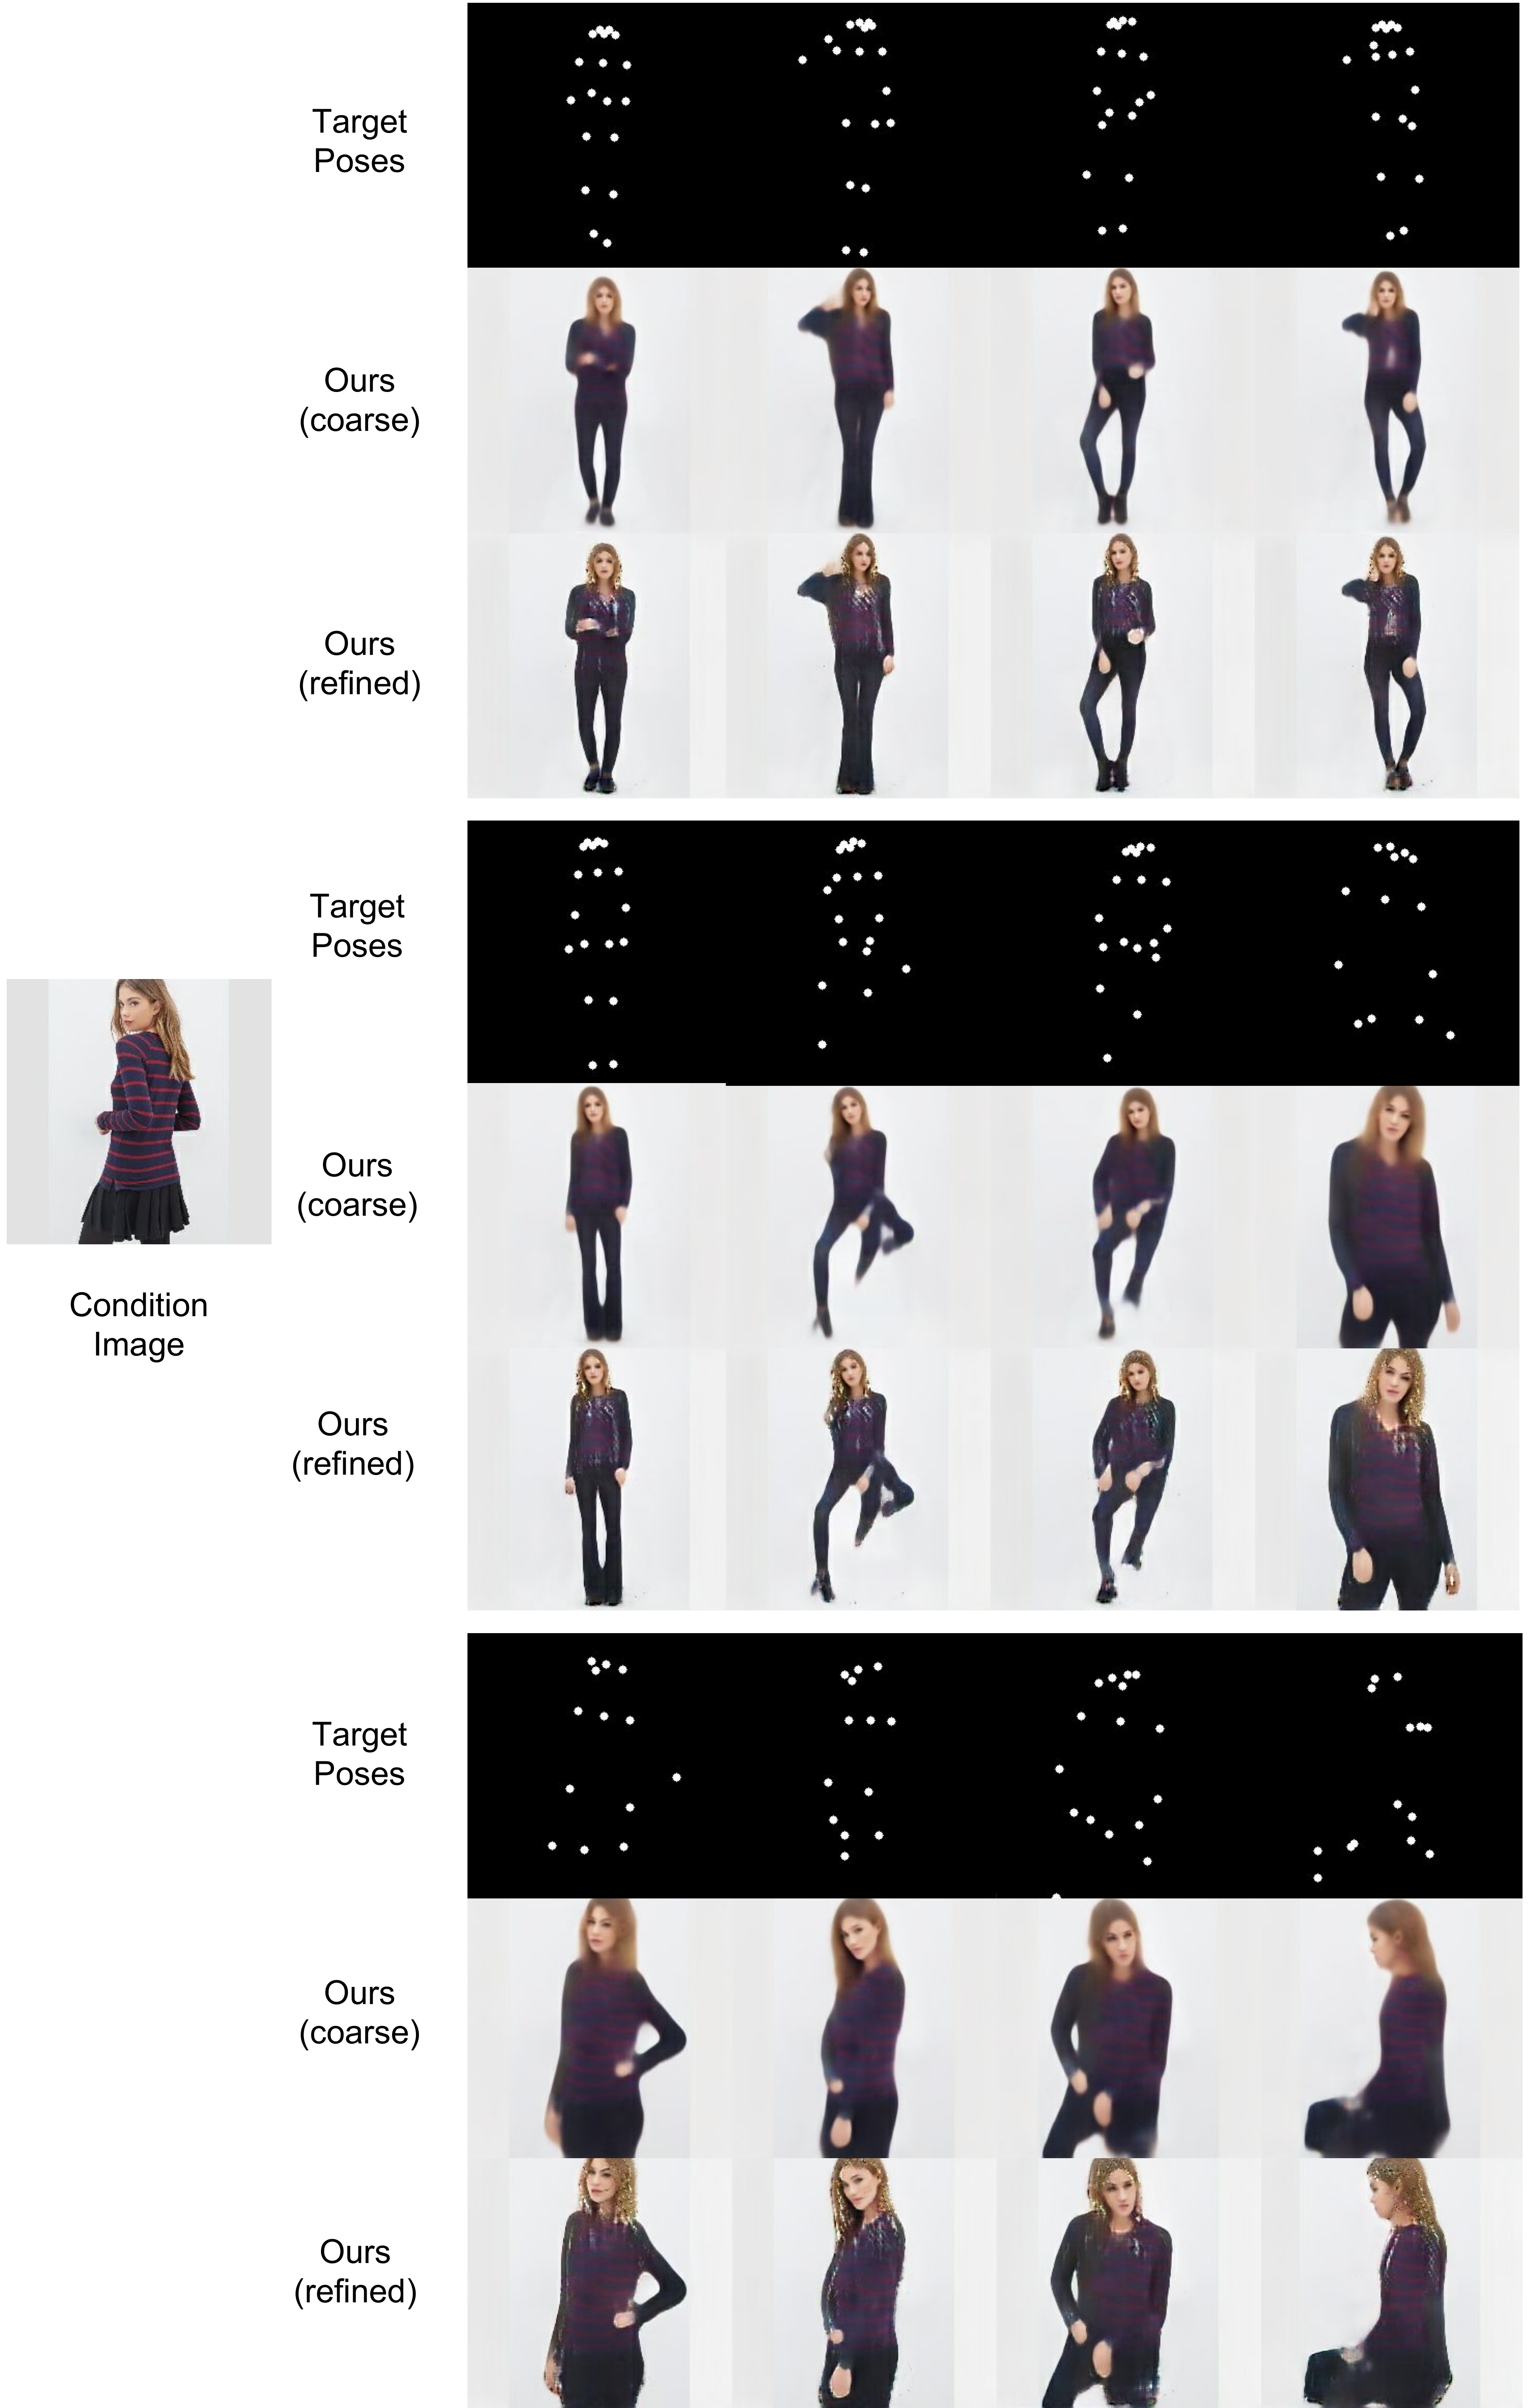}
  \caption{Generated results for one person with various target poses on the DeepFashion dataset.}
  \vspace{-0.2cm}
  \label{seq_df1}
\end{figure}

\begin{figure}
\centering
  \includegraphics[width=\linewidth]{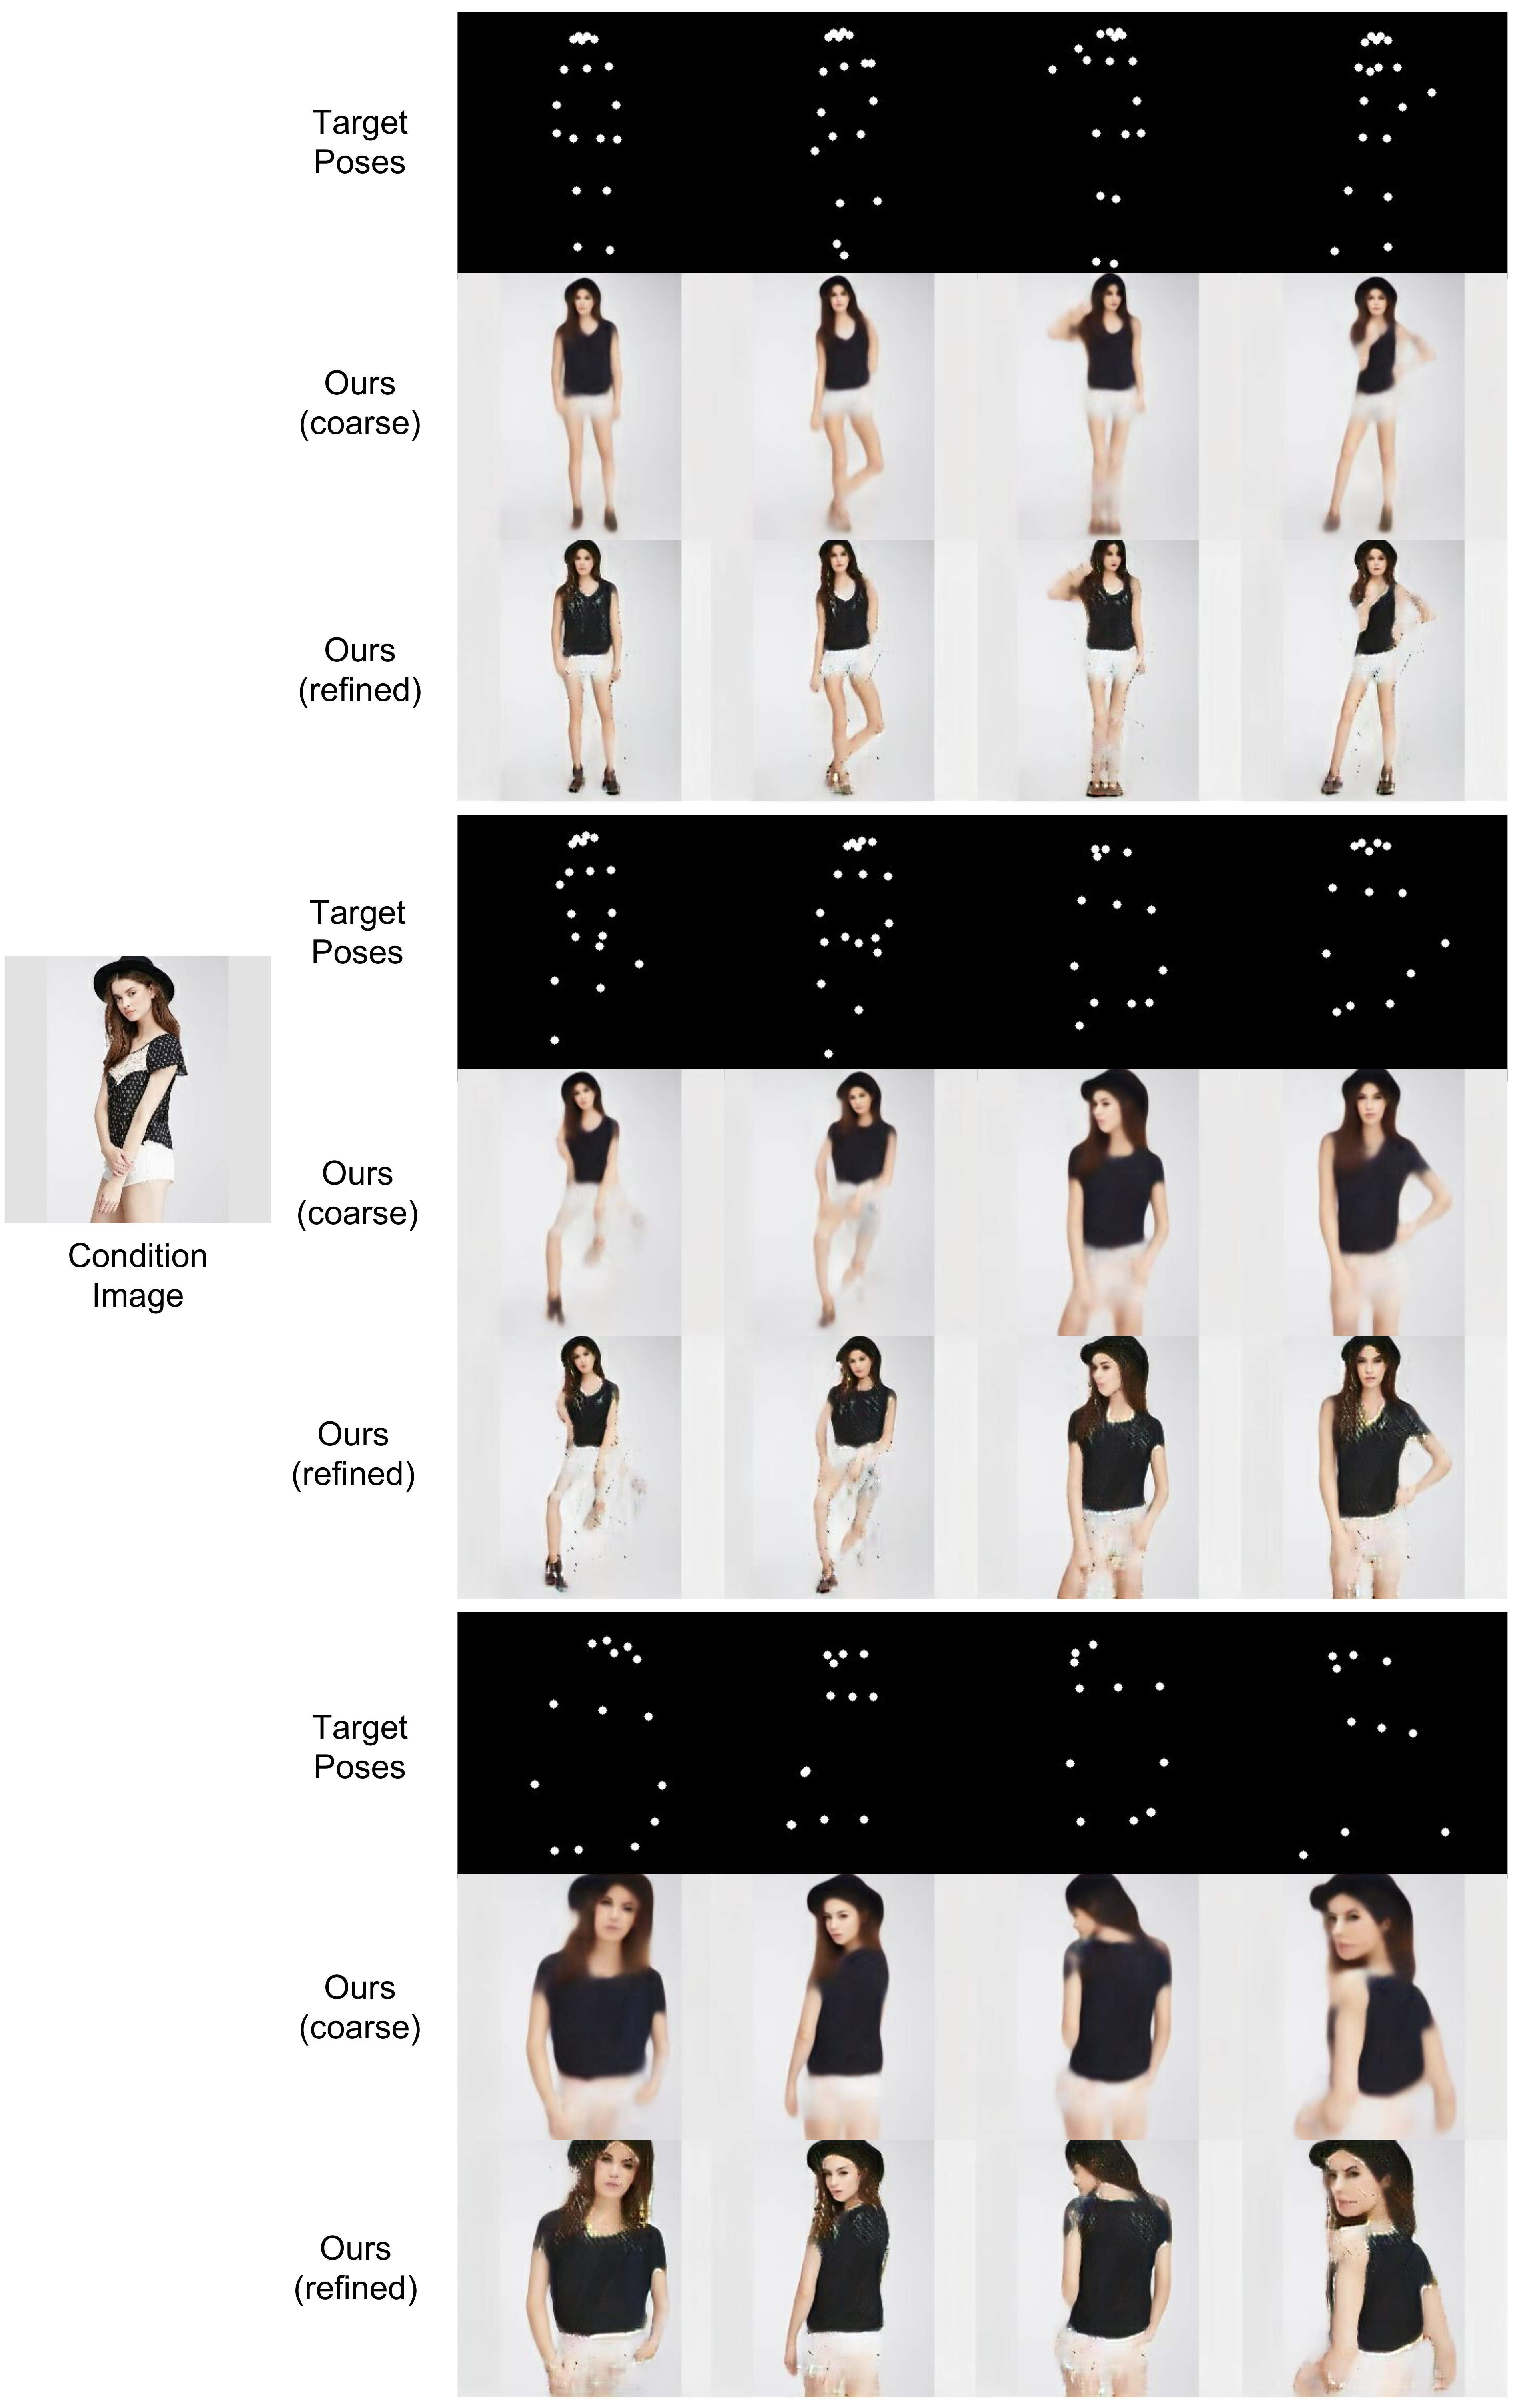}
  \caption{Generated results for one person with various target poses on the DeepFashion dataset.}
  \vspace{-0.2cm}
  \label{seq_df2}
\end{figure}

\begin{figure}
\centering
  \includegraphics[width=\linewidth]{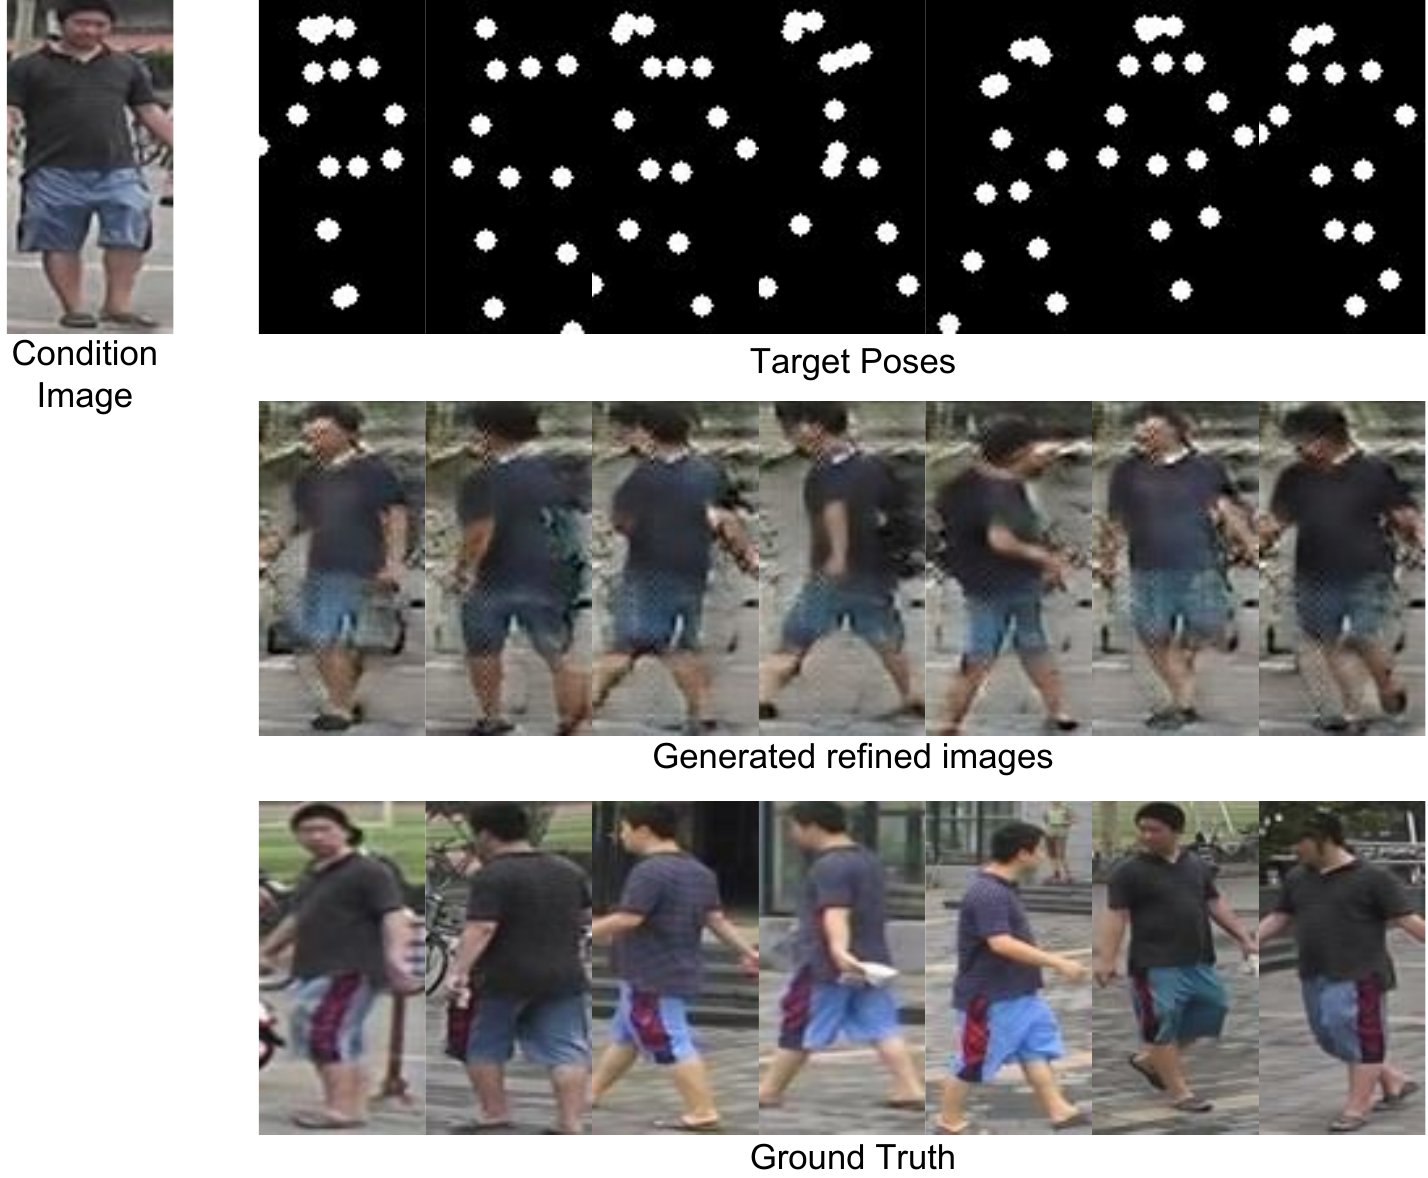}
  \caption{Generated results for one person with various target poses on the Market-1501 dataset.}
  \vspace{-0.2cm}
  \label{seq_market}
\end{figure}

In this section, we give more generation results conditioned on one person image and a set of different poses. Note that these poses are computed by a pose estimator on random person images in the dataset.
From Figure~\ref{seq_df1} and~\ref{seq_df2},~\ref{seq_market}, we can see our model is able to generate photo-realistic results conditioned on multiple poses.
