# Supplementary material for: Pose Guided Person Image Generation
Source: arXiv:1705.09368 source file (2018-01-28)
Supplement: Supplementary file 4 [file 4-supp-good.tex]

\section{Generated results}
\label{supp-good}
In Figure~\ref{good_DF} and Figure~\ref{good_market}, we show more pose guided person image generation results.

\begin{figure}[th]
\centering
  \includegraphics[width=1\linewidth]{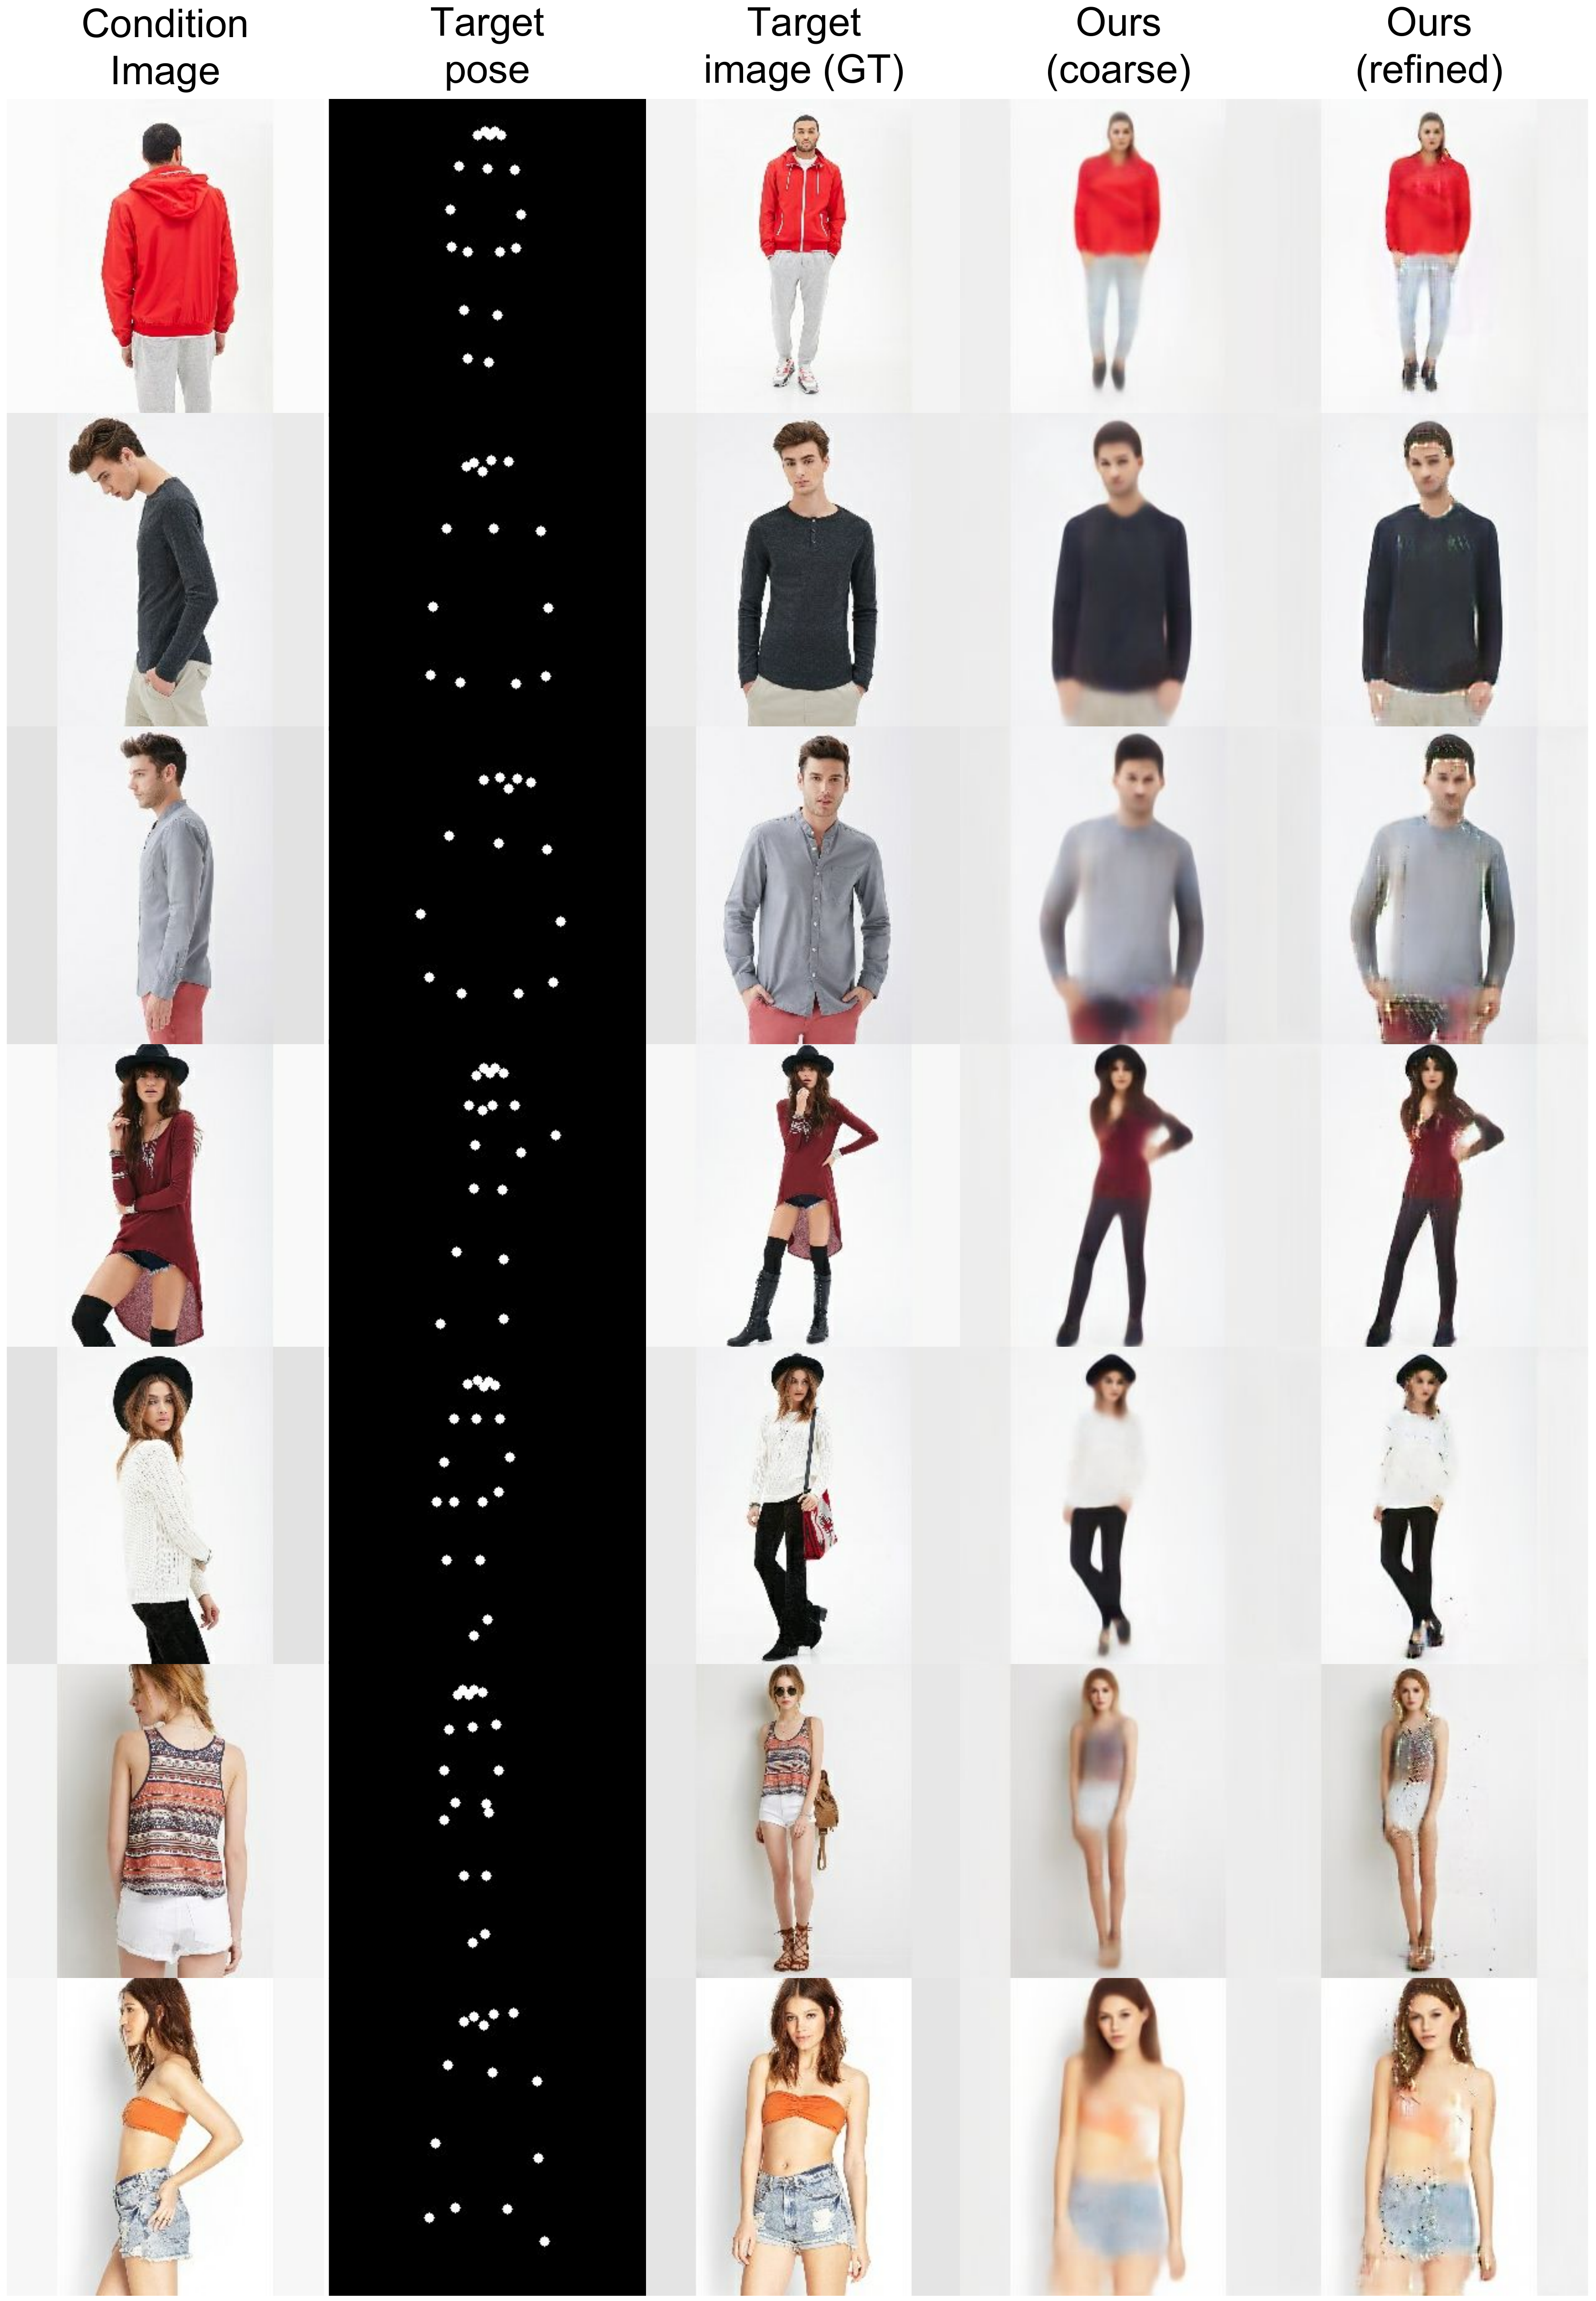}
  \caption{Generated results on the DeepFashion dataset.}
  \label{good_DF}
\end{figure}

\begin{figure}[th]
\centering
  \includegraphics[width=0.8\linewidth]{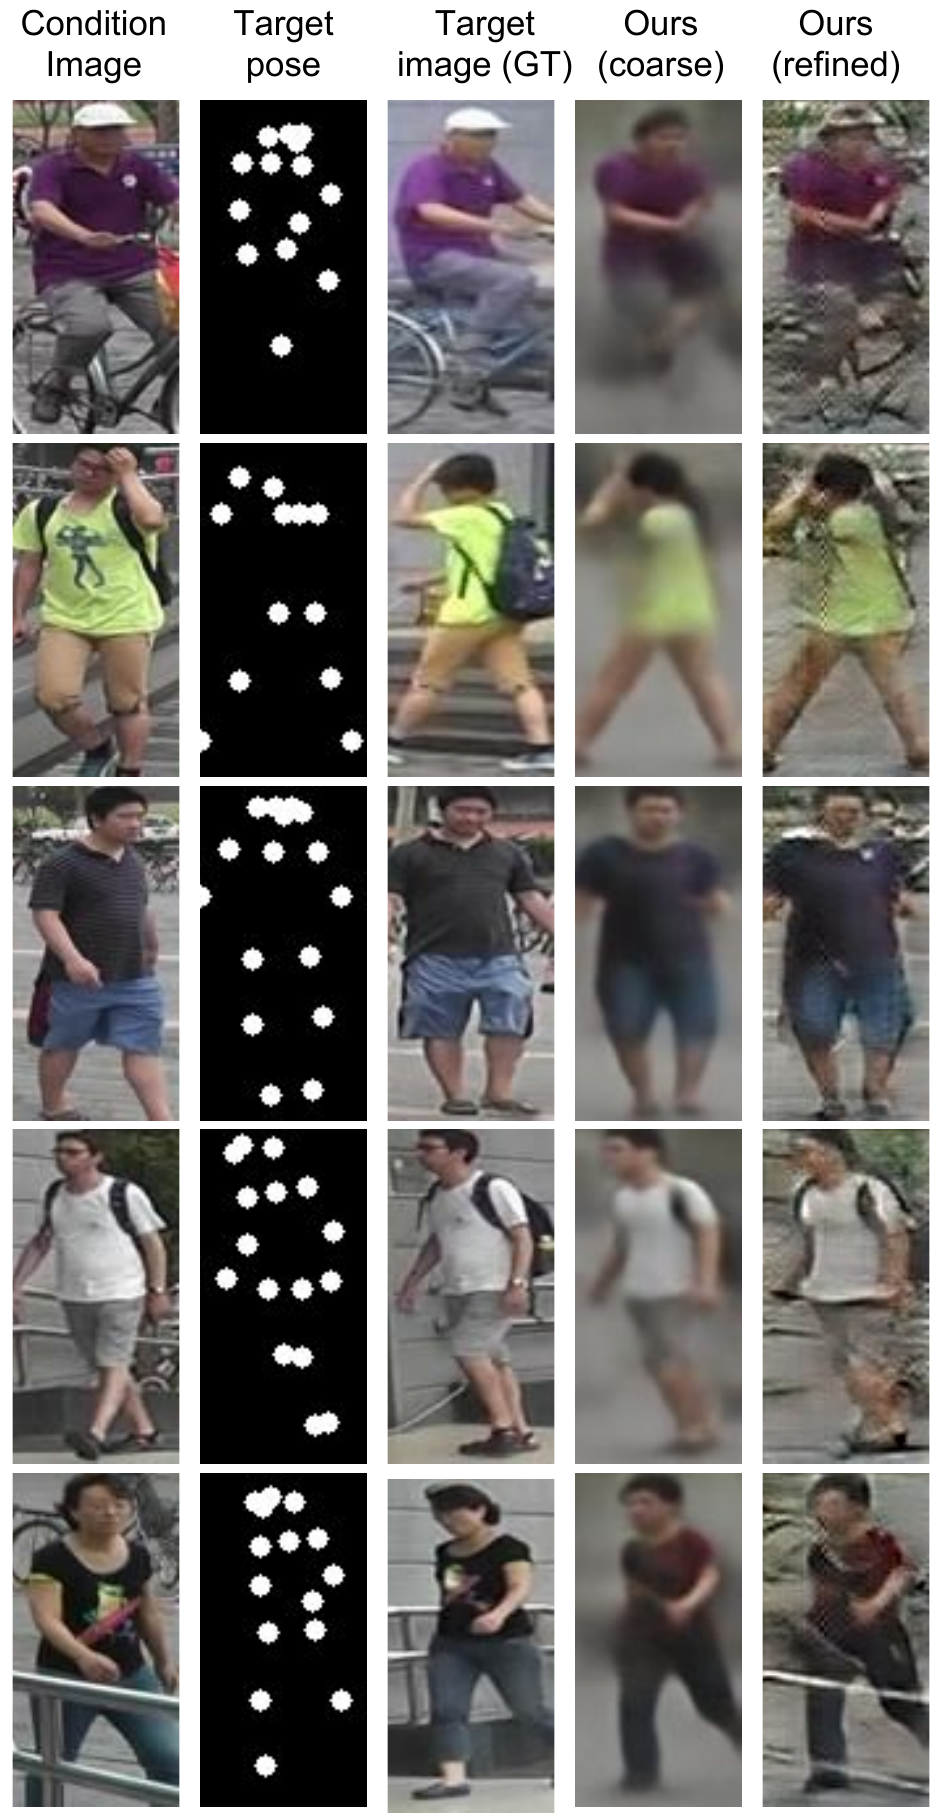}
  \caption{Generated results on the Market-1501 dataset.}
  \label{good_market}
\end{figure}
