# Supplementary material for: Pose Guided Person Image Generation
Source: arXiv:1705.09368 source file (2018-01-28)
Supplement: Supplementary file 5 [file 5-supp-bad.tex]

\section{Failure results}
\label{supp-bad}
In figure~\ref{seq_failure2} and Figure~\ref{seq_failure1}, we show some failure cases of our method. The main reasons of failure cases include dramatic scale change, inaccurate pose input, and the rare case of samples.

\begin{figure}[th]
\centering
  \includegraphics[width=1\linewidth]{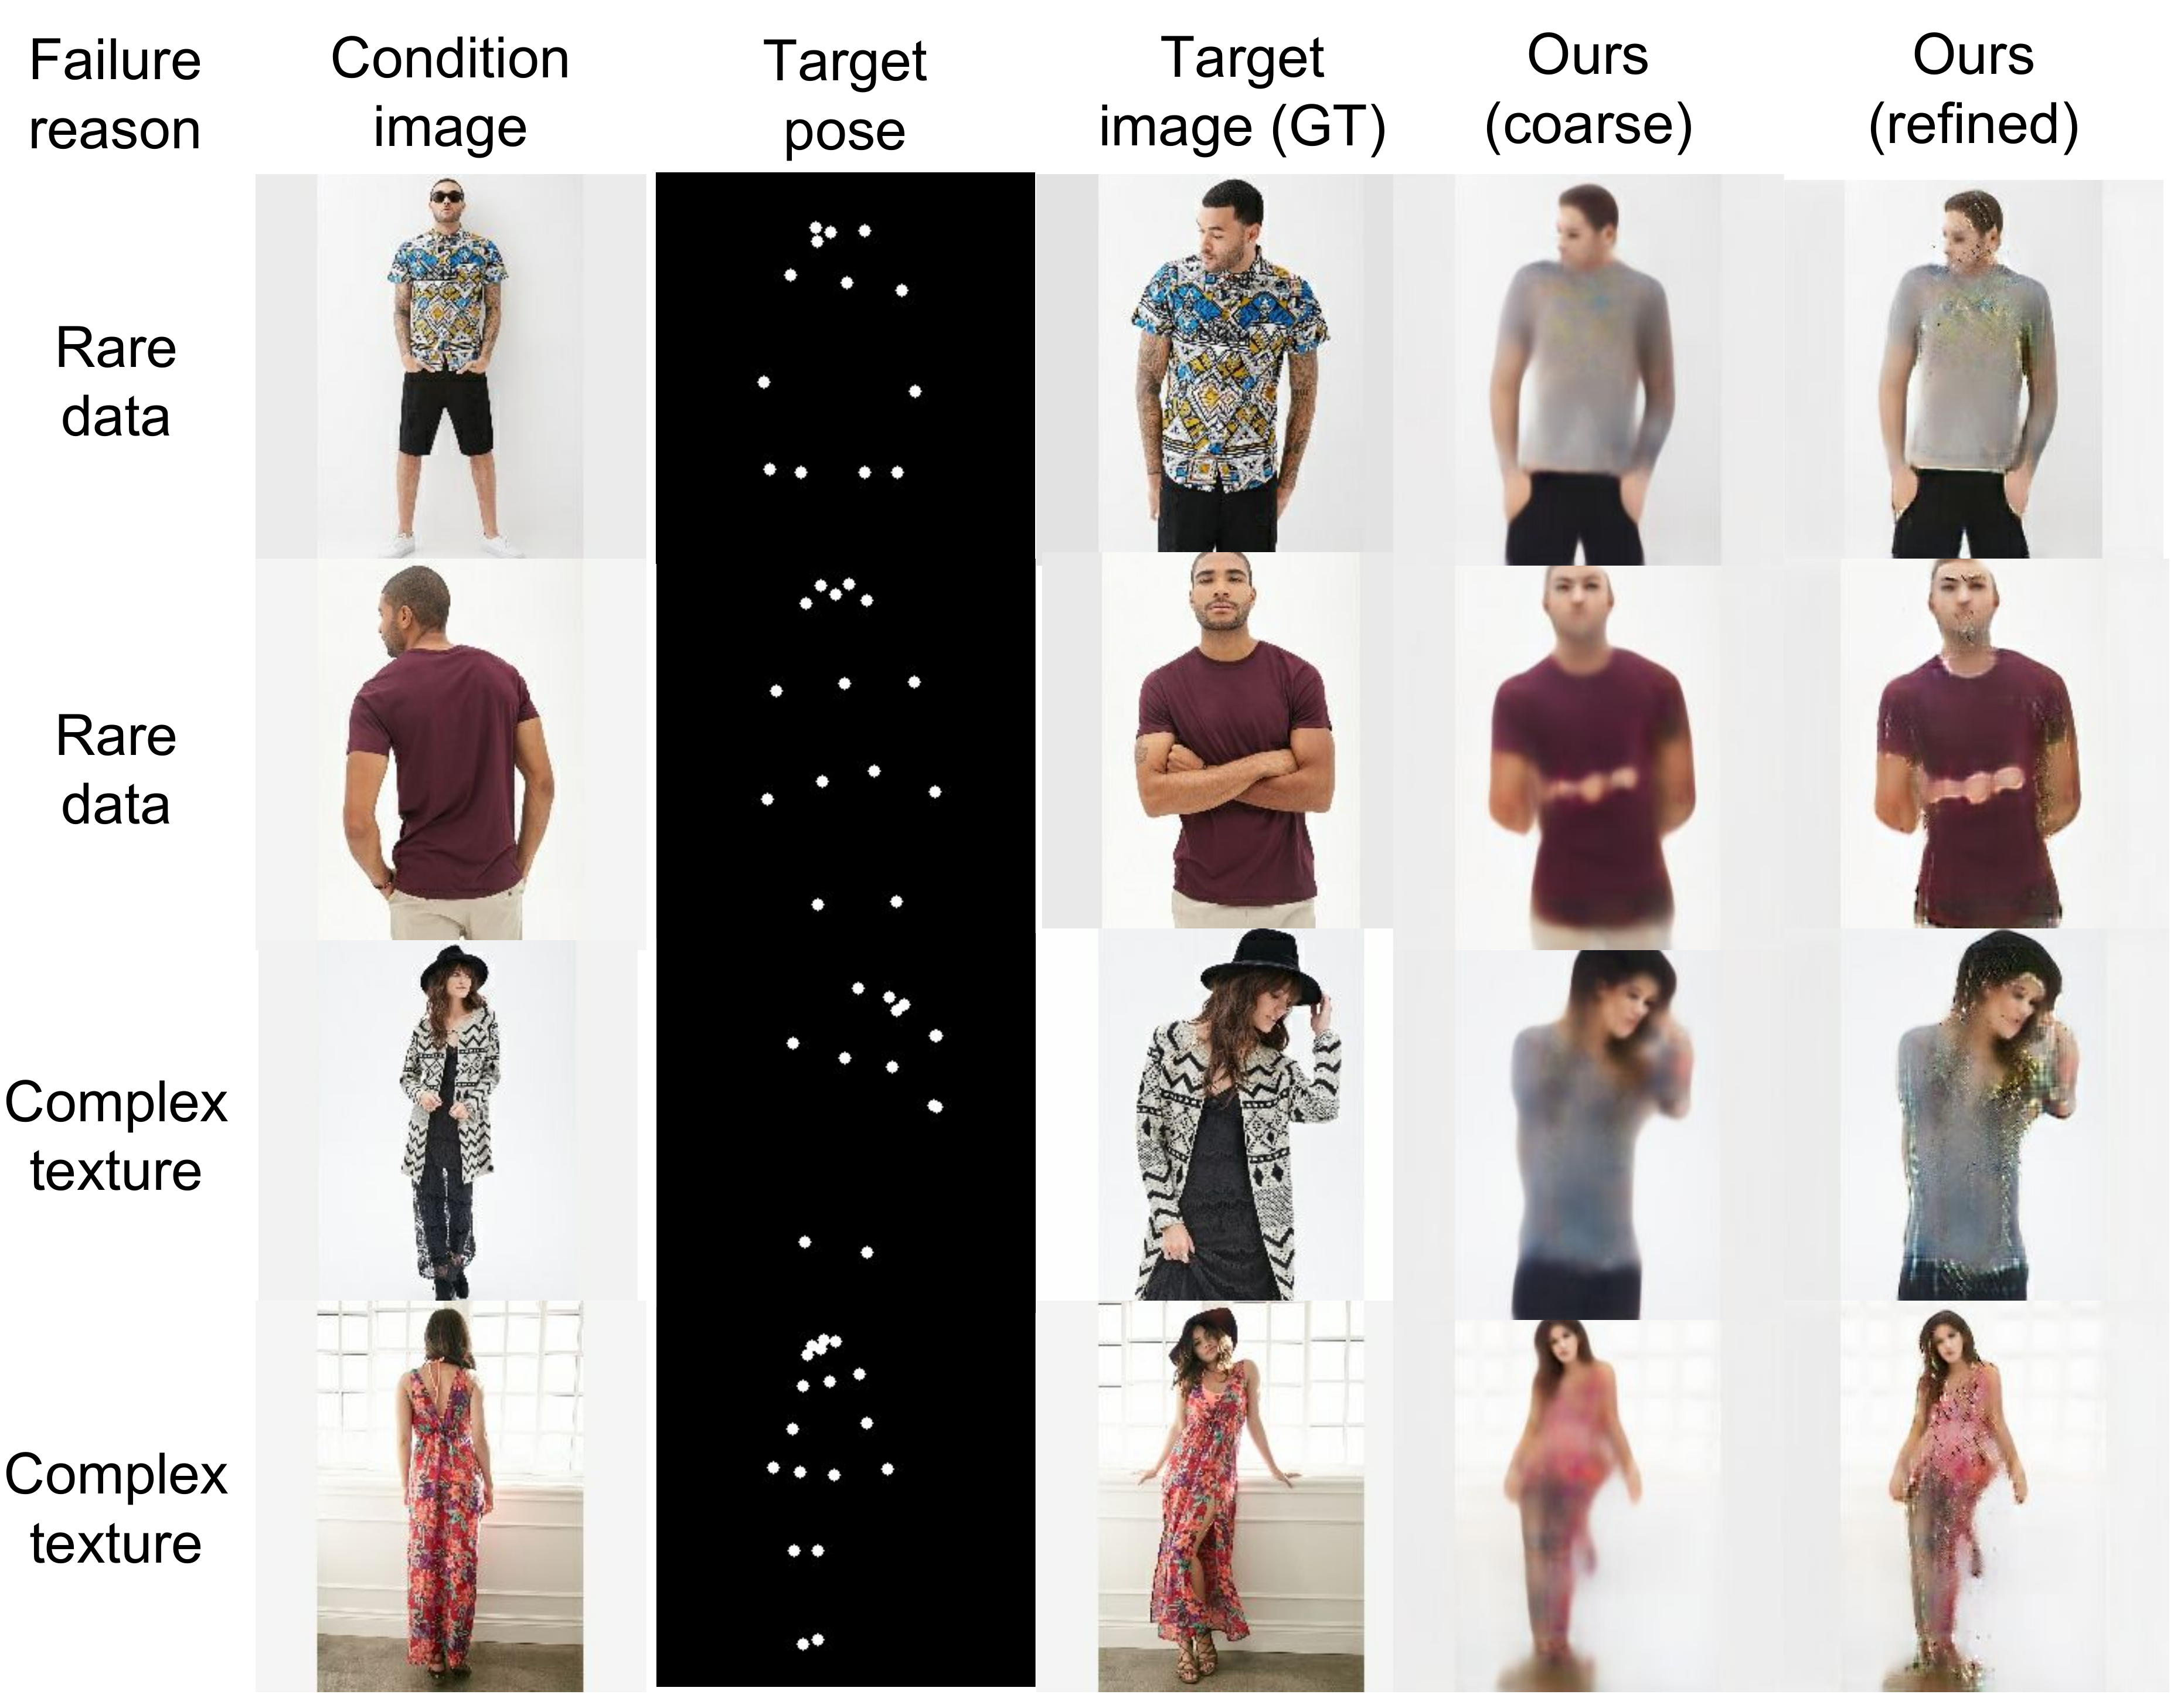}
  \caption{Failure cases on the DeepFashion dataset.}
  \label{seq_failure2}
\end{figure}

\begin{figure}[th]
\centering
  \includegraphics[width=0.9\linewidth]{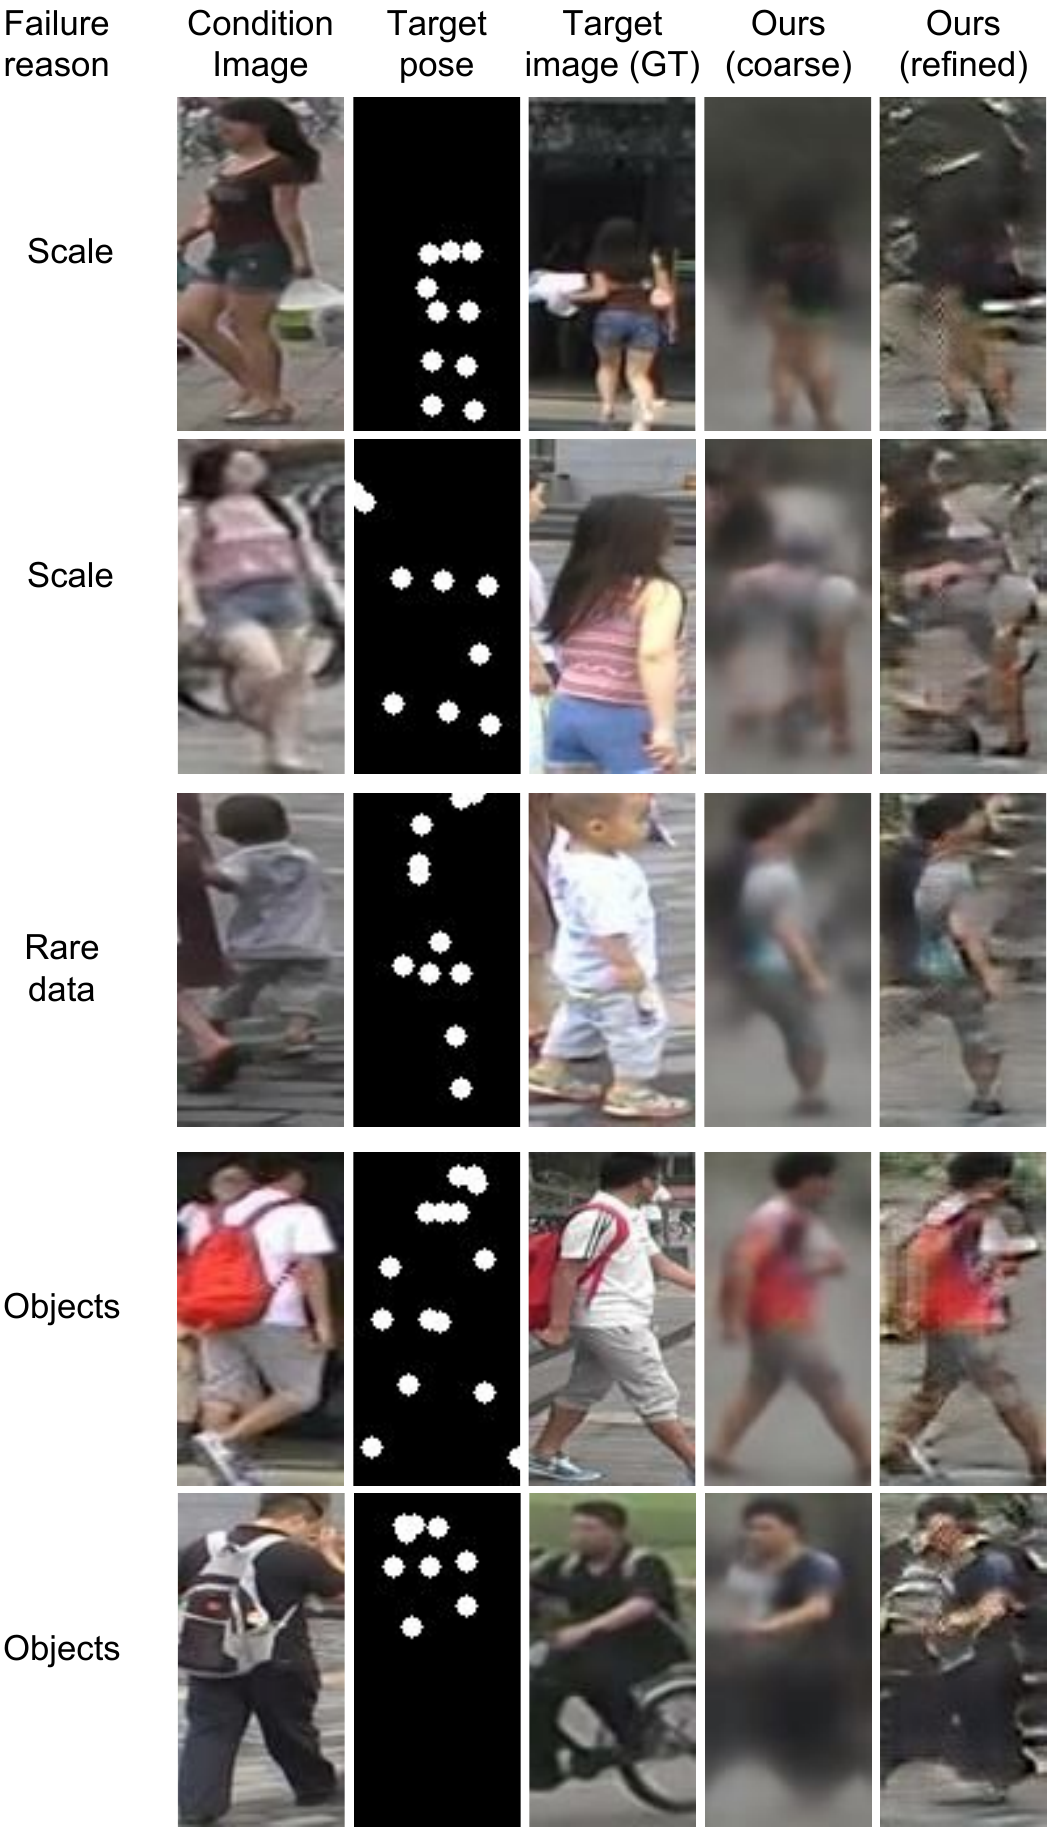}
  \caption{Failure cases on the Market-1501 dataset.}
  \label{seq_failure1}
\end{figure}
